# Supplementary material for: AR-1-to-3: Single Image to Consistent 3D Object Generation via Next-View Prediction
Source: arXiv:2503.12929 source file (2025-08-09)
Supplement: Supplementary file 1 [file X_suppl.tex]

\clearpage
\setcounter{page}{1}
\maketitlesupplementary
% \onecolumn
\appendix

\section{More Ablative Results}

\myPara{Ablation on Local Feature Encoding.}
When the length of the view sequence becomes excessively long, the Stacked-LE strategy may encounter GPU burden issues. 
Inspired by recent works in video generation~\cite{zhou2024storydiffusion}, we introduce a random sampling design to alleviate this concern. 
Specifically, we retain all $L$ tokens of $e_{i}^{1}$ as they originate from the input image, and perform random sampling with a proportion of $\alpha$ on the L tokens from each generated novel view. 
When the $\alpha$ value is set to 0, the Stacked-LE strategy degenerates to the original Reference attention; when $\alpha$ is 1, it is equivalent to using all tokens as in \maineqn{2} of the main text.

We investigate the impact of $\alpha$ on the performance and efficiency of our model in a train-free fashion.
We freeze the trained model parameters and calculate the two measure values, \ie PSNR and FLOPS, at different sampling rates.
As shown in \figref{fig:abl_ratio}, the PSNR value drops sharply when $\alpha$ is 0.
We believe that the reason is that the parameters of \nMethod{} have been optimized based on additional view features.
If the model misses them, ambiguity may arise in understanding 3D objects.
When $\alpha$ is greater than 0, the PSNR value gradually increases with $\alpha$.
Meanwhile, the FLOPS value, which we calculate according to the maximum autoregressive sequence length, continues to increase.
%
% In this paper, we set the $\alpha$ value to 1 by default.
%
To achieve a trade-off between performance and efficiency, it is recommended to take a $\alpha$ value between 0.3 and 1 based on the sequence length and GPU resources.
%

% \myPara{Discussion on Error Accumulation Issue of AR Theme.}

\section{More Visualization Results}
Apart from the quantitative and qualitative evaluation in the main text, we also provide more visualization examples from the benchmark dataset, \ie Objaverse~\cite{deitke2023objaverse}, and the out-of-domain dataset, \ie GSO~\cite{downs2022google} and Omni3D~\cite{wu2023omniobject3d}, to further validate the effectiveness of our \nMethod{}.
%
% 文字物体，人形物体，多物体，

\myPara{Novel View Synthesis.}
We select three types of hard cases , including word-object, humanoid-object, and multi-object, to highlight the superiority of the proposed next-view prediction paradigm for novel view synthesis.
As shown in \figref{fig:suppl_view_syn_word}, \figref{fig:suppl_view_syn_humanoid}, and \figref{fig:suppl_view_syn_mo}, the novel views progressively generated by our \nMethod{} (blue boxes) can capture intricate geometric and textural details of various complex objects, closely mirroring the given images (black boxes).

\myPara{Image-to-3D Generation.}
As shown in \figref{fig:suppl_ito3d}, our \nMethod{} can produce high-quality 3D objects that adhere to diverse and complex image prompts, which should be attributed to the consistent novel views generated by our next-view prediction.
These results demonstrate that assigning different generation priorities based on the camera poses difference between novel views and the input view is a promising paradigm towards high-fidelity 3D asset creation.

\section{Future Work}
This work establishes a next-view prediction paradigm for consistent novel view synthesis and 3D asset creation.
However, constrained by computational resources, several promising research directions remain unexplored and are reserved for future work.
\textbf{1) Scalability.} To obtain more powerful 3D generation capabilities, we plan to curate a larger collection of high-quality 3D data from ObjaverseXL and replace our SD diffusion model with DiT.
\textbf{2) Training Optimization.} To better facilitate next-view prediction modeling, we intend to upgrade the supervision from the views of current views to the total view sequence.
\textbf{2) Method Extension.} We will explore to extend the proposed next-view prediction paradigm from Zero123++ to other multi-view diffusion models, \eg ImageDream~\cite{wang2023imagedream}.

\myinputfig{abl_ratio}

\myinputfig{suppl_view_syn_word}
\myinputfig{suppl_view_syn_humanoid}

\myinputfig{suppl_view_syn_mo}
\myinputfig{suppl_ito3d}
