# Supplementary material for: AR-1-to-3: Single Image to Consistent 3D Object Generation via Next-View Prediction
Source: arXiv:2503.12929 source file (2025-08-09)
Supplement: Supplementary file 2 [file suppl_ito3d.tex]

\begin{figure*}[t]
    \centering
    \footnotesize
    \includegraphics[width=0.98\linewidth]{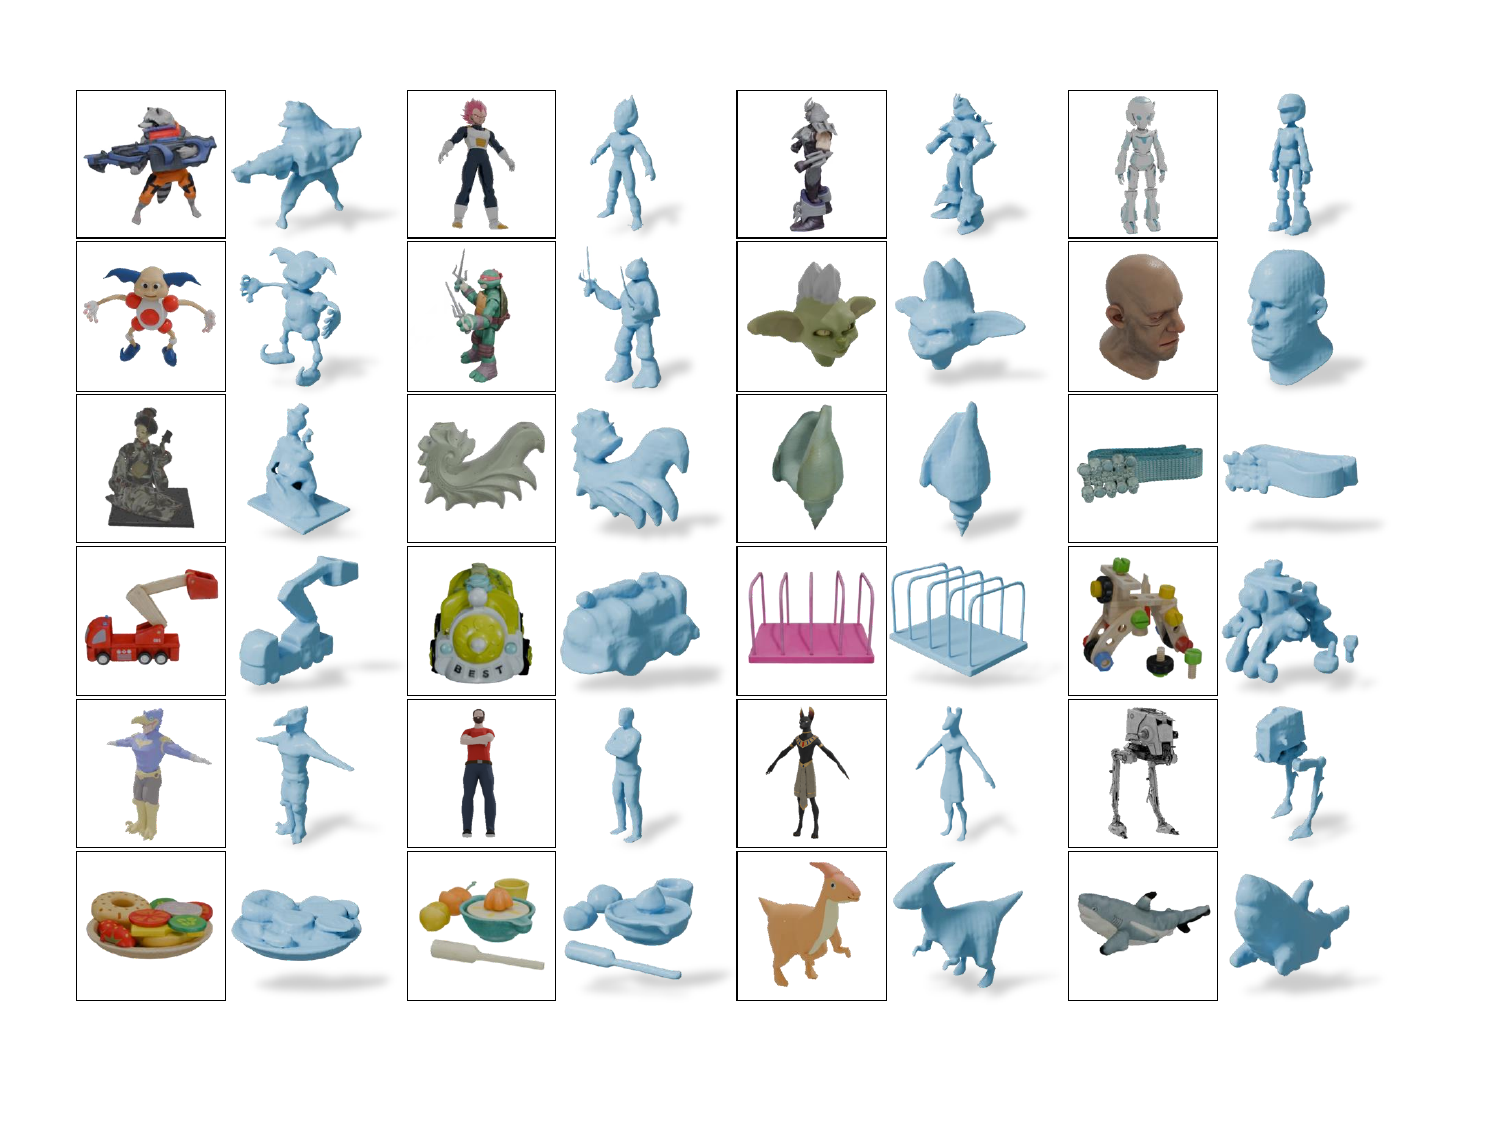}
    % \fbox{\rule[-.5cm]{0cm}{5cm} \rule[-.5cm]{13cm}{0cm}}
    \vspace{-3pt}
    \caption{Visualization results of the proposed \nMethod{} model on more image-to-3d examples.}
    \label{fig:suppl_ito3d}
    \vspace{-10pt}
\end{figure*}
