# Supplementary material for: AR-1-to-3: Single Image to Consistent 3D Object Generation via Next-View Prediction
Source: arXiv:2503.12929 source file (2025-08-09)
Supplement: Supplementary file 3 [file suppl_view_syn_humanoid.tex]

\begin{figure*}[t]
    \centering
    \footnotesize
    \includegraphics[width=0.98\linewidth]{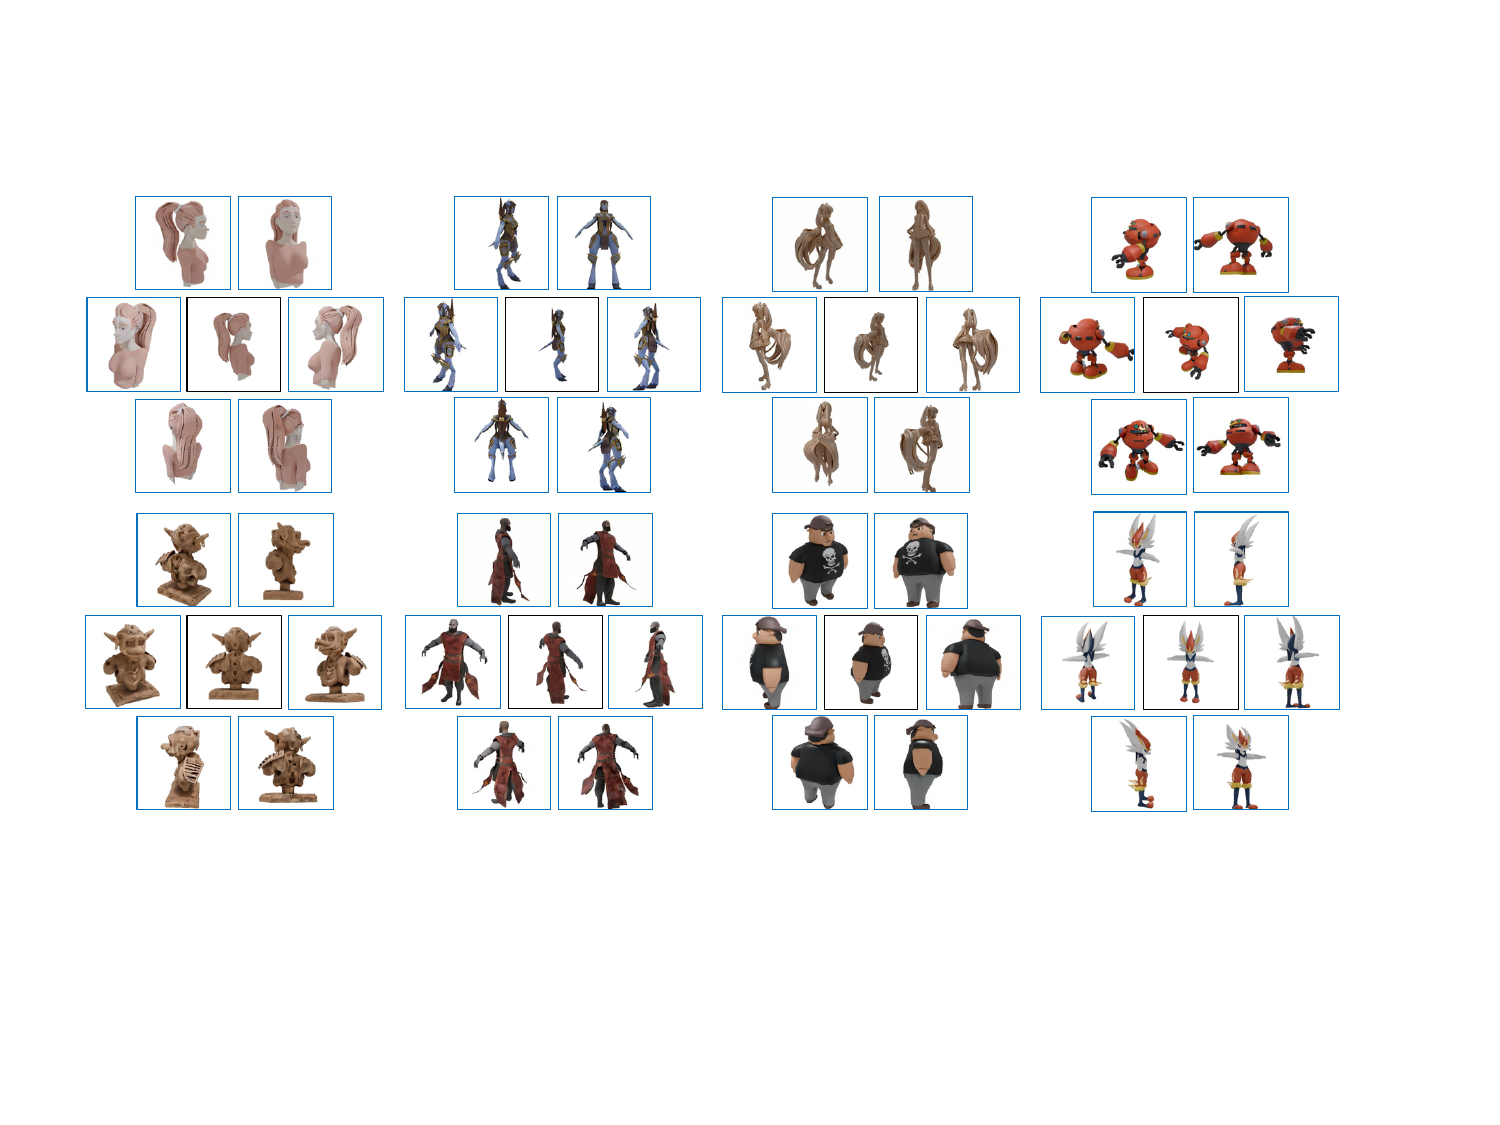}
    % \fbox{\rule[-.5cm]{0cm}{5cm} \rule[-.5cm]{13cm}{0cm}}
    % \vspace{-7pt}
    \caption{
    Visualization results of the proposed \nMethod{} model on novel view synthesis of humanoid-object examples.}
    \label{fig:suppl_view_syn_humanoid}
    % \vspace{-10pt}
\end{figure*}
