# Supplementary material for: AR-1-to-3: Single Image to Consistent 3D Object Generation via Next-View Prediction
Source: arXiv:2503.12929 source file (2025-08-09)
Supplement: Supplementary file 4 [file suppl_view_syn_mo.tex]

\begin{figure*}[t]
    \centering
    \footnotesize
    \includegraphics[width=0.98\linewidth]{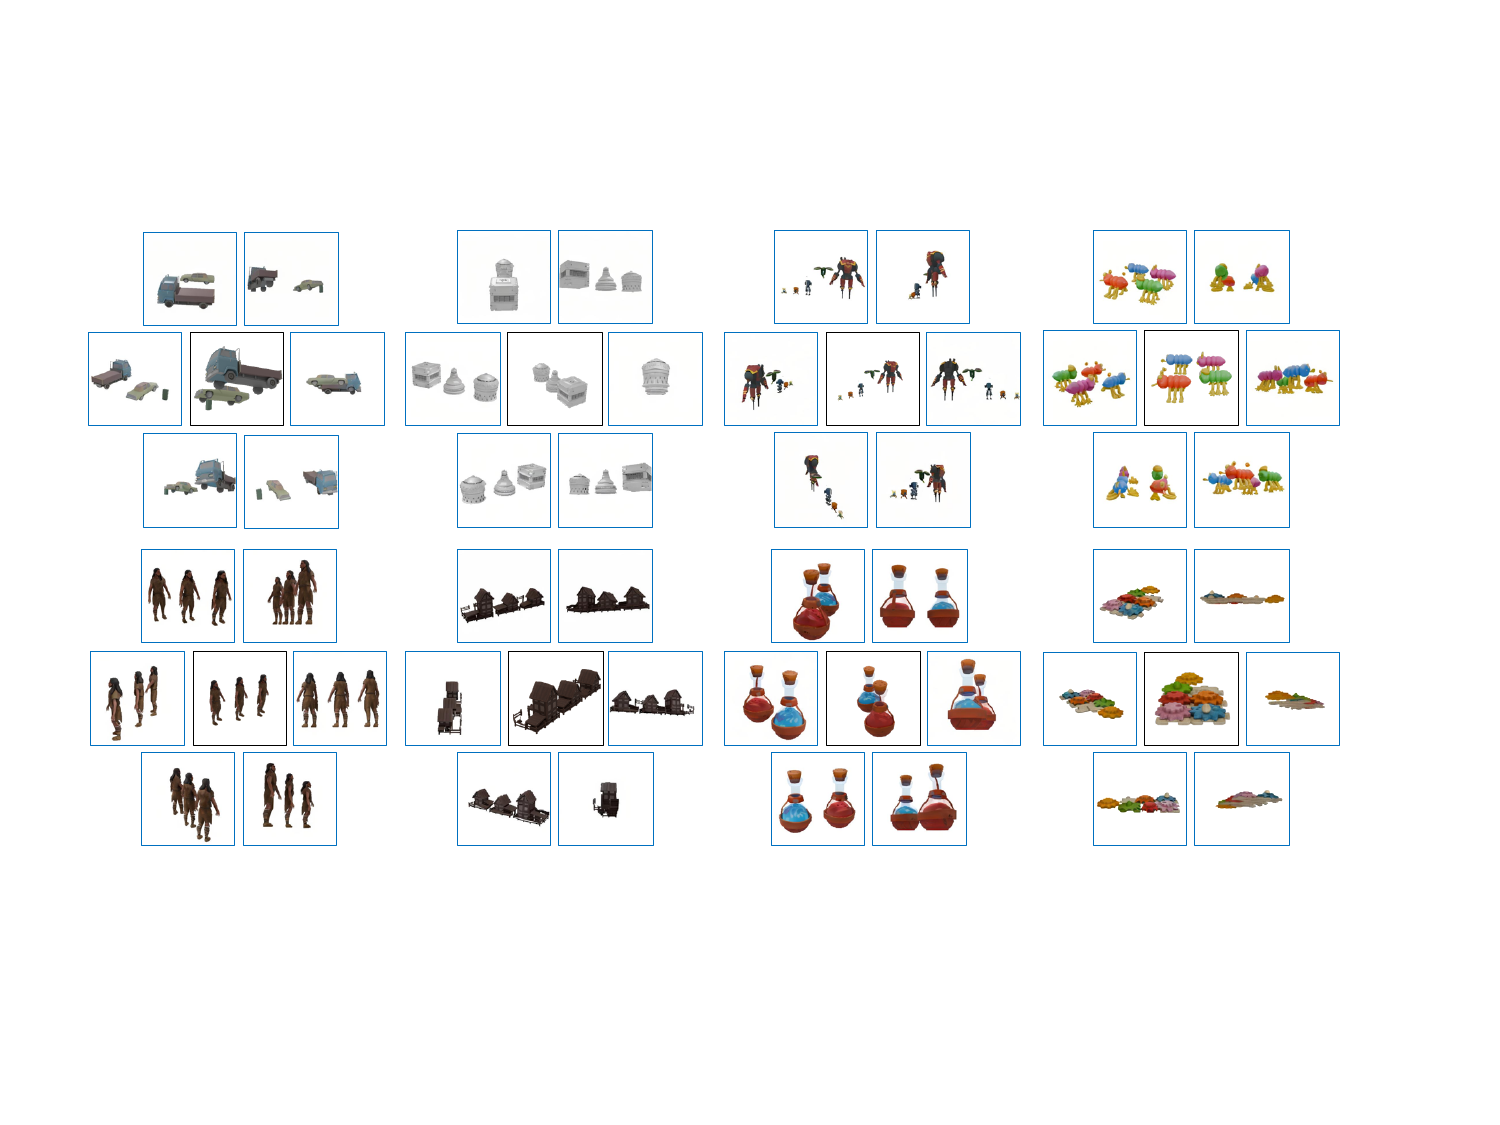}
    % \fbox{\rule[-.5cm]{0cm}{5cm} \rule[-.5cm]{13cm}{0cm}}
    \vspace{-3pt}
    \caption{
    Visualization results of the proposed \nMethod{} model on novel view synthesis of multi-object examples.}
    \label{fig:suppl_view_syn_mo}
    \vspace{5pt}
\end{figure*}
